# Supplementary material for: U.S. Power Resilience for 2002--2019
Source: arXiv:2103.15859 ancillary file (2021-07-20)
Supplement: Supplementary file 3 [file readme.pdf]

# Power Resiliency

This README file is provided as supplementary material to the research article.

## data\_cleaning.R

### Objective

This script will clean the datasets and load in environment variables. It should always be run first. The script also contains some experimental code including producing maps but can be ignored. The file should be used for data cleaning purposes. To experiment with influential points, modify the boolean `remove_influential_rows` on line 156.

### Required files

The following datasets used to run this program were manually modified as noted in the article.

- EIA-861 files from 'datasets/EIA and OE datasets' folder. Original data: [EIA-861](#). Download will be a .zip and the relevant file is Sales\_Ult\_Cust\_XXXX, where XXXX is the year. Keep in Excel format.
- OE-417 files from 'datasets/EIA and OE datasets' folder Original data: [OE-417](#). Save the files as Tab Delimited Text (txt).

### Other requirements

- Ensure that data files are placed in the same directory and that you change the working directory in the script to point to the directory which contains the files.
- Ensure that the packages required are installed:

```
lubridate
readxl
plyr
ggplot2
xlsx
ggpubr
dplyr
usmap
BBmisc
scales
```

## us\_maps.R

### Objective

This script will create the US choropleth maps that illustrate various combinations of year, reliability metric, and cause of outage for each state. It creates three XLSX files (SAIDI, CAIDI, SAIFI) used for the Lasso analysis as well.

### Required files

data\_cleaning.R

## Other requirements

- Each time this file is run, data\_cleaning.R must execute successfully prior to ensure the correct environment values are loaded.
- Ensure that the packages required are installed:

```
dplyr
usmap
gridExtra
xlsx
extrafont
```

## line\_graphs.R

### Objective

This script will create the line graphs that illustrate various combinations of year, reliability metric, NERC region, and cause of outage. It also calculates the influence measures for California.

### Required files

- EIA-861 dataset
- OE-417 dataset
- NERC\_regions.xlsx from 'datasets/' folder

## Other requirements

- run us\_maps.R
- Ensure that the packages required are installed:

```
plyr
dplyr
readxl
openxlsx
lubridate
ggplot2
extrafont
gridExtra
sqldf
```

## for\_regression.R

### Objective

This script will create the prepare part of the data to required for the Lasso analysis.

### Required files

- Areas of States.csv
- outage.xlsx
- NERC\_regions.xlsx from 'datasets/' folder

### Other requirements

- No other file is required to run prior.
- Ensure that the packages required are installed:

```
dplyr  
extrafont  
gridExtra  
usmap  
xlsx
```

## lasso\_analysis.Rmd

### Objective

This script will conduct the LASSO regression analysis based on the provided predictor variables dataset. It also includes experimental trials involving step regression using AIC and BIC criteria.

### Required files

- for\_regression.csv
- CAIDI.xlsx
- SAIDI.xlsx
- SAIFI.xlsx

### Other requirements

- No other file is required to run prior.
- Ensure that the packages required are installed:

```
MASS  
glmnet  
stargazer
```
